# Supplementary material for: Efficient Routing Algorithm Design for Large DetNet
Source: arXiv:2303.00527 source file (2023-03-01)
Supplement: Supplementary file 1 [file appendix3_not_used.tex]

\section{Srlg Selection Strategies}\label{appendix:srlg_strategy}
In line 13 of Algorithm \ref{algorithm:conflict_pulse_plus}, an Srlg selection strategy is required. In order to reduce the size of the resulting conflict set, we tried the following two heuristic Srlg-selection strategies:
\begin{description}
    \item[Strategy 1:] Pick the Srlg $r\in \Omega(P_{s\rightarrow t})\cap \Omega(P_a)$ that contains the largest number of links.
    \item[Strategy 2:] Find the first link $e\in P_a$ such that $\Omega(P_{s\rightarrow t})\cap \Omega(e)\neq\emptyset$, and then pick the Srlg $r\in \Omega(P_{s\rightarrow t})\cap \Omega(e)$ that contains the largest number of links.
\end{description}

We compare the two Srlg-selection strategies using all the problem instances in the test sets Srlg-DRCR\_1 and Srlg-DRCR\_2 (see Section \ref{sec:generate_test_cases}). In Figure \ref{fig:conflict_set_strategy_compare1} and \ref{fig:conflict_set_strategy_compare2}, we compare the distribution of the conflict set size under both Srlg-selection strategies. The total number of conflict sets generated for all the problem instances is $83,380$ and $149,251$ for Strategy 1 and Strategy 2, respectively. The average size of each conflict set generated by Strategy 1 is also smaller than that generated by Strategy 2. In Figure \ref{fig:conflict_set_strategy_compare3}, we compare the solver running time of the CoSE-Pulse$+$ algorithm (we have enabled joint cost \& delay pruning). We can see that Strategy 1 reduces the largest solver running time by about $1-54046/100971 \approx 46.5\%$ when compared with Strategy 2. Based on the above analysis, we choose the first one as our default Srlg-selection strategy.

%Our observation is that the conflict sets generated by the second Srlg-selection strategy are larger than those generated by the first one on average and the total scale is also larger, which means it takes longer to traverse the conflict sets but the larger conflict set doesn't help reduce the complexity of the problem. From Figure \ref{fig:conflict_set_strategy_compare2}, 

\begin{figure}[!h]
    \centering
    \subfigure[Distribution of the Conflict Set Size of Strategy 1.] {
        \label{fig:conflict_set_strategy_compare1}
        \includegraphics[scale=0.35]{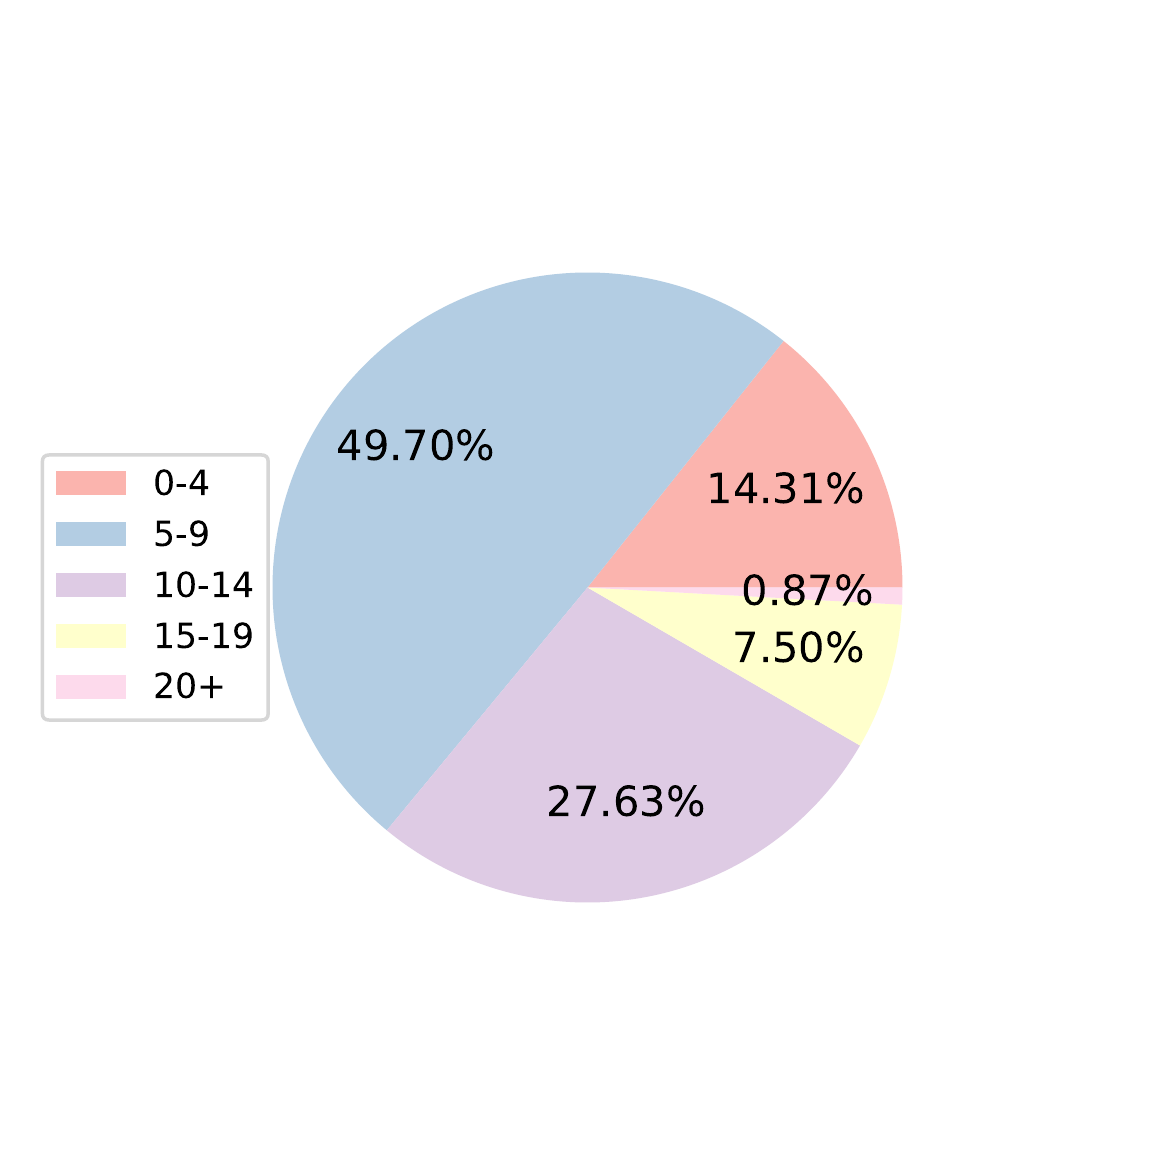}
    }
        \subfigure[Distribution of the Conflict Set Size of Strategy 2.] {
        \label{fig:conflict_set_strategy_compare2}
        \includegraphics[scale=0.35]{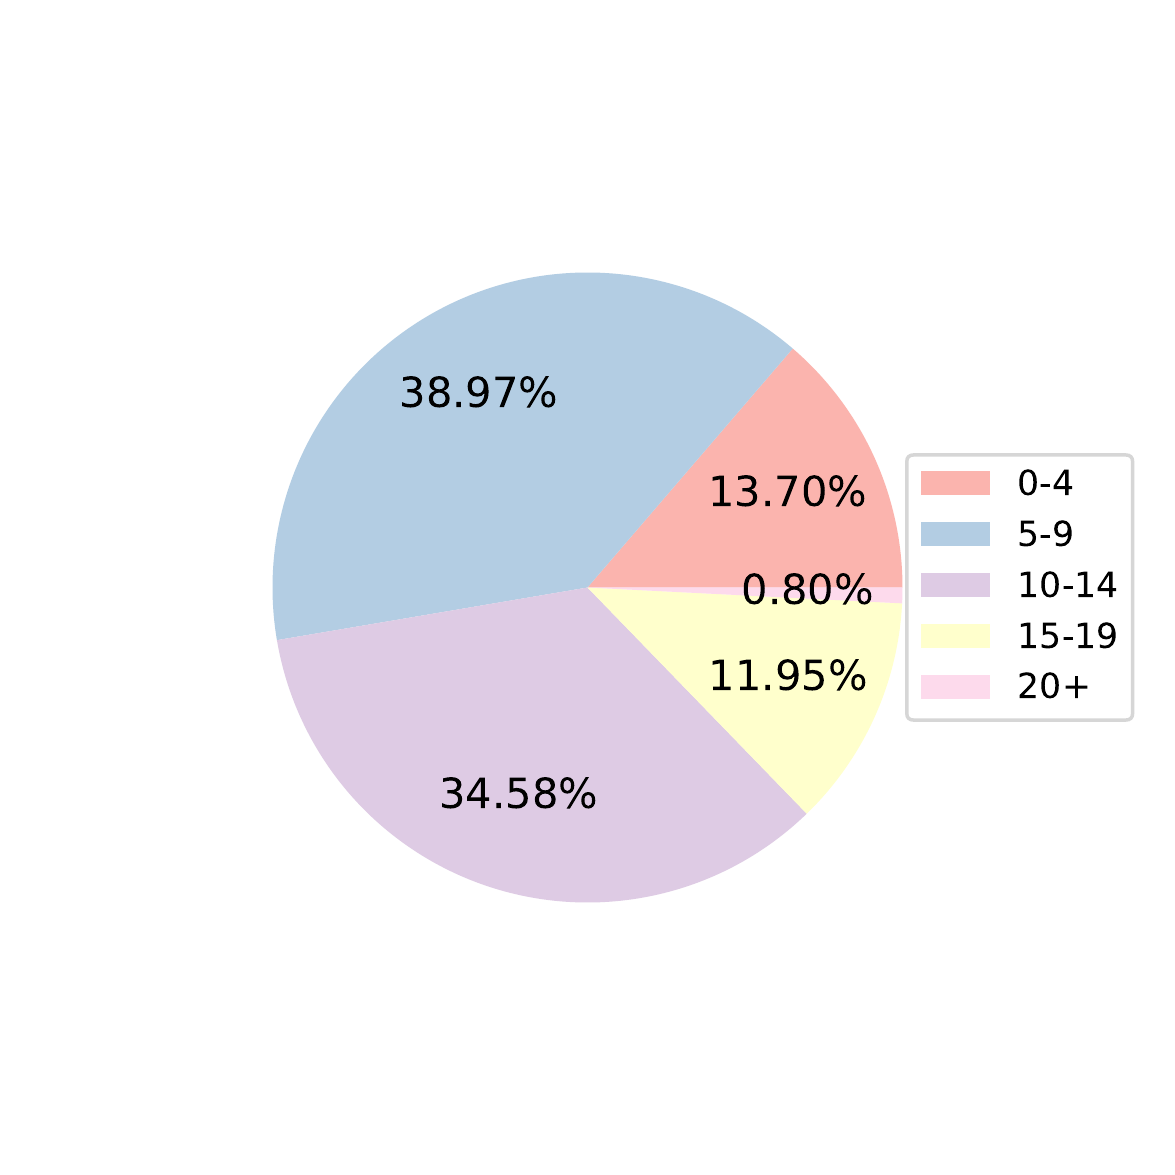}
    }
    \hspace{4mm}
    \subfigure[CoSE-Pulse$+$ Running Time under both Srlg Selection Strategies.] {
        \label{fig:conflict_set_strategy_compare3}
        \includegraphics[scale=0.5]{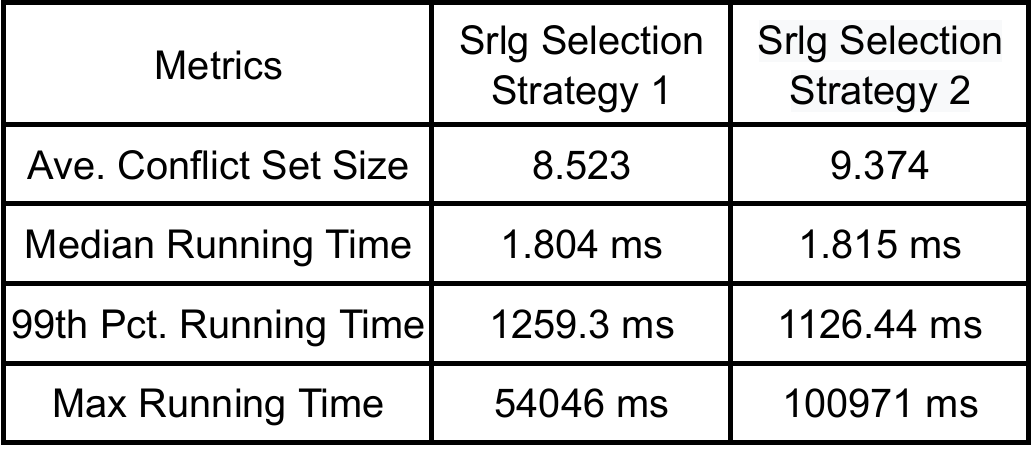}
    }
    \caption{Compare two Srlg selection strategies using the two test sets Srlg-DRCR\_1 and Srlg-DRCR\_2. Since all the test cases are feasible, the size of each conflict set is at least 2.}
    \label{fig:conflict_set_strategy_compare}
\end{figure}

\subsection{A heuristic approach}
We adopt a heuristic approach \cite{ribeiro1985a} here. This approach divide the $N$ into three partition $\{N_1,N_f,N_2\}$ such that $s\in N_1$ and $t \in N_2$. Then the graph $G$ can be divided into $G_1(G_2)$ induced by $N_1 \cup N_f(N_f\cup N_2)$ with arc set $E_1(E_2)$. The path $P$ from $s$ to $t$ can be combined by \emph{partial solution} $P_1$ and \emph{final solution} $P_2$, where $P_1$ is the paths from $s$ to $j\in N_f$ which takes only arcs of $E_1$ and $P_2$ is the paths from $j\in N_f$ to $t$ which takes only arcs of $U_2$. The algorithm is based on a systematic way of generating a subset of partial solution and combining them with all final solution(obtained by enumeration). Algorithm \ref{algorithm:generate the subset of partial solution} is shown how to generate the subset of partial solution. Some mathematical proofs are proposed to ensure the correctness of algorithm \ref{algorithm:generate the subset of partial solution}, you can get more details in \cite{ribeiro1985a}. Let $[P_A(\lambda)]$ denote the problem of calculating the shortest path tree $A(\lambda)$ from $s$ to all nodes of $N_1 \cup N_f$, with respect to the lengths $c+\lambda d$. Let $P_1(j,\lambda)$ denote the the shortest path from $s$ to $j$. For $u=(i,j)$, let $d_1(A(\lambda,u))=c(P_1(i,\lambda)) + c(u) - c(P_1(j,\lambda)), d_2(A(\lambda,u))=d(P_1(i,\lambda)) + d(u) - d(P_1(j,\lambda))$. And denote by $F(A(\lambda),i)$ be the set of nodes $k$ of $N_1 \cup N_f$ such that the node $i$ belongs to the path from $s$ to $k$ within $A(\lambda)$. Equation \ref{eqn:positive delta}, \ref{eqn:negetive delta} and \ref{eqn:update solution tree} is used in algorithm \ref{algorithm:generate the subset of partial solution}.
\begin{equation}\label{eqn:positive delta}
\delta_u = \left\{
\begin{array}{cc}
     -d_1(A(\lambda),u)/d_2(A(\lambda),u),  &d_2(A(\lambda),u)<0,  \\
     +\infty, &otherwise.
\end{array}\right.\ \lambda>0
\end{equation}
\begin{equation}\label{eqn:negetive delta}
\delta_u = \left\{
\begin{array}{cc}
     -d_1(A(\lambda),u)/d_2(A(\lambda),u),  &d_2(A(\lambda),u)>0,  \\
     -\infty, &otherwise.
\end{array}\right.\ \lambda<0
\end{equation}
\begin{equation}
\label{eqn:update solution tree}
\begin{split}
&c(P_1(k,A(\overline{\lambda})))=\left\{
\begin{array}{cc}
    c(P_1(k,A(\lambda)))+d_1(A(\lambda),\Bar{u}),& if\ k\in F(A(\lambda),j),  \\
     c(P_1(k,A(\lambda))),& otherwise, 
\end{array}
\right.\\
&d(P_1(k,A(\overline{\lambda})))=\left\{
\begin{array}{cc}
    d(P_1(k,A(\lambda)))+d_2(A(\lambda),\Bar{u}),& if\ k\in F(A(\lambda),j),  \\
     d(P_1(k,A(\lambda))),& otherwise, 
\end{array}
\right.\\
&F(A(\overline{\lambda}),k)) = F(A(\lambda),k), k\neq i\ and\ k \neq l, \\
&F(A(\overline{\lambda}),i)) = F(A(\lambda),i) \cup  F(A(\lambda),j),\\
&F(A(\overline{\lambda}),l)) = F(A(\lambda),l)-F(A(\lambda),j)
\end{split}
\end{equation}
\begin{algorithm}[h]
\SetAlgoLined
\KwData{A network $G(V,E)$, node subset $\{N_1,N_f\}$, edge subset $E_1$, and a delay range $[L,U]$.}
\KwResult{the subset of partial solution $\mathcal{P}$.}
Define a min heap $H_{min}$ to get the positive breakpoint. Initially, $H_{min}$ is empty;\\
Define a max heap $H_{max}$ to get the negative breakpoint. Initially, $H_{max}$ is empty;\\
Initially $\lambda=0$, and solve the problem $[P_A(\lambda)]$ obtaining the tree $A(\lambda)$ as its solution.\\
\For{every $j\in N_f$}
{
$\mathcal{P}_j \leftarrow \mathcal{P}_j \cup \{P_1(j,\lambda)\}$;\\
}
\For{every $e\in E_1$}{
Compute $\delta_u$ by equation \ref{eqn:positive delta};\\
$H_{min}.\text{push}.(\delta_u)$;
}
$\overline{\lambda} = \delta_{\Bar{u}}=\min_{u\in U_1}\{\delta_u\}$;\\
\While{$\lambda \neq +\infty$}{
Let $A_{\Bar{u}}(\lambda)$ be the graph obtained from the solution $A(\lambda)$ by inserting $\Bar{u}=(i,j)$ and deleting $v=(l,j)$ in original $A(\lambda)$.\\
\If{$A_{\Bar{u}(\lambda)}$ is a tree}
{
    The solution $A(\overline{\lambda})=A_{\Bar{u}}(\lambda)$ of problem $[P_A(\overline{\lambda})]$ can be got by equation \ref{eqn:update solution tree};\\
    \For{every $j\in N_f$}
    {
    $\mathcal{P}_j \leftarrow \mathcal{P}_j \cup \{P_1(j,\lambda)\}$;\\
    }
    \For{every $e=(a,b)\in E_1$ such that $a\in F(A(\overline{\lambda}),j)$ or $b\in F(A(\overline{\lambda}),j)$}{
    Compute $\delta_u$ by equation \ref{eqn:positive delta};\\
    $H_{min}.\text{push}.(\delta_u)$;
    }
    $\overline{\lambda} = \delta_{\Bar{u}}=\min_{u\in U_1}\{\delta_u\}$;\\
}\Else{break;}
}
$\lambda = 0$, and obtain the tree $A(\lambda)$;\\
\For{every $e\in E_1$}{
Compute $\delta_u$ by equation \ref{eqn:negetive delta};\\
$H_{max}.\text{push}.(\delta_u)$;
}
$\overline{\lambda} = \delta_{\Bar{u}}=\max_{u\in U_1}\{\delta_u\}$;\\
then do the similar operation in line 12-28, just use equation \ref{eqn:negetive delta} to compute $\delta_u$, and change $H_{min}$ to $H_{max}$.
\caption{Generate the subset of partial solution}
\label{algorithm:generate the subset of partial solution}
\end{algorithm}

\section{Joint Pruning for Pulse$+$}\label{appendix:joint_pruning}
We propose an enhancement method for the pruning strategies of Pulse$+$. For every node $u$, we define a cost function $f_u:\mathbb{R}^+\rightarrow\mathbb{R}^+$ that maps from delay budget to path cost, and use this function to prune a branch $P_{s\rightarrow u}$ if the following condition is met:
\begin{equation}\label{eqn:joint_delay_cost_prune}
\boxed{c(P_{s\rightarrow u})+f_u(L-d(P_{s\rightarrow u}))\geq\text{tmp\_min}.}
\end{equation}
Then, we have the following theorem.

\begin{theorem}\label{lem:joint_delay_cost_prune}
Assume that the cost function $f_u(l)$ satisfies the following two conditions for all $$l=L-d(P_{s\rightarrow u})\in (-\infty, L-d(P_{s\rightarrow u}^{\text{min\_delay}})].$$
%\todo{Assume that the cost function$f_u(l)$(l can be any value, but here, $l = L-d(P_{s\rightarrow u})$ to represent the gap between $L$ and $d(P_{s\rightarrow u})$)satisfies:} 
\begin{enumerate}
    \item $f_u(l)=+\infty$ if there exists no elementary path $P_{u\rightarrow t}$ from $u$ to $t$ satisfying $l\leq d(P_{u\rightarrow t})\leq l+U-L$;
    \item $f_u(l)\leq c(P_{u\rightarrow t})$ for any elementary path $P_{u\rightarrow t}$ from $u$ to $t$ satisfying $l\leq d(P_{u\rightarrow t})\leq l+U-L$.
\end{enumerate}
Then, if a branch $P_{s\rightarrow u}$ satisfies the constraint (\ref{eqn:joint_delay_cost_prune}), searching this branch will not yield a solution with end-to-end cost lower than $\text{tmp\_min}$.
\end{theorem}

\begin{proof}
The proof is straightforward. If $f_u(L-d(P_{s\rightarrow u}))=+\infty$, then (\ref{eqn:joint_delay_cost_prune}) always holds. In this case, there does not exist an elementary path $P_{u\rightarrow t}$ such that $L\leq d(P_{s\rightarrow u}) + d(P_{u\rightarrow t})\leq U$. Therefore, the branch $P_{s\rightarrow u}$ can be safely cut.

If $f_u(L-d(P_{s\rightarrow u}))<+\infty$, then for any elementary path $P_{u\rightarrow t}$ satisfying $L\leq d(P_{s\rightarrow u})+d(P_{u\rightarrow t})\leq U$, we must have $c(P_{s\rightarrow u})+c(P_{u\rightarrow t})\geq c(P_{s\rightarrow u})+f_u(L-d(P_{s\rightarrow u}))\geq\text{tmp\_min}$. In this case, searching the branch $P_{s\rightarrow u}$ will not yield a solution with end-to-end cost lower than $\text{tmp\_min}$, and thus this branch can be safely cut.
\end{proof}

The strength of the pruning strategy (\ref{eqn:joint_delay_cost_prune}) depends on the cost function $f_u$. Consider the following cost function:
\begin{equation}\label{eqn:cost_function_example}
f_u(l)=\left\{
\begin{aligned}
&+\infty, & \text{ if }l< d(P_{u\rightarrow t}^{\text{min\_delay}})-U+L, \\
&c(P_{u\rightarrow t}^{\text{min\_cost}}), & \text{ if }l\geq d(P_{u\rightarrow t}^{\text{min\_delay}})-U+L.
\end{aligned}
\right.
\end{equation}
It is easy to verify that the pruning strategy (\ref{eqn:joint_delay_cost_prune}) degenerates to the original pruning strategy (\ref{eqn:prune_strategy}).

In order to obtain better pruning effect, we need a tighter cost function. Obviously, the tightest cost function is \begin{equation}\label{eqn:opt_cost_function}
f_u(l)=\min_{P_{u\rightarrow t}\text{ is elementary and } d(P_{u\rightarrow t})\in [l, l+U-L]} c(P_{u\rightarrow t}).
\end{equation}
However, calculating the above cost function requires solving a large number of DRCR problems, which is computationally expensive. To reduce the algorithmic complexity, we compute the following relaxed cost function instead:
\begin{equation}\label{eqn:relaxed_cost_function}
f_u(l)=\min_{P_{u\rightarrow t}\text{ is a path satisfying } d(P_{u\rightarrow t})\in [l, l+U-L]} c(P_{u\rightarrow t}).
\end{equation}
Clearly, the cost function in (\ref{eqn:relaxed_cost_function}) satisfies the conditions in Lemma \ref{lem:joint_delay_cost_prune}. The key difference between (\ref{eqn:relaxed_cost_function}) and (\ref{eqn:opt_cost_function}) is that (\ref{eqn:relaxed_cost_function}) does not require a path $P_{u\rightarrow t}$ to be elementary. As we will see shortly, this relaxation enables a revised dominance check to cut searching branches, making (\ref{eqn:relaxed_cost_function}) much more easier to calculate than (\ref{eqn:opt_cost_function}).

% greatly reduces the computational complexity and also enjoys good performance.

\subsubsubsection{Calculating the Relaxed Cost Functions (\ref{eqn:relaxed_cost_function})}\label{subsubsection:calculate_cost_function}

\noindent\textbf{A Revised Dominance Check:} For every path $P$ ($P$ may contain cycles), we can obtain a delay-cost pair $(d(P),c(P))$. We first propose a revised dominance check as follows:
\begin{definition}\label{def:revised_dominance_check}
Given two partial paths $P_{u\rightarrow t}^1$ and $P_{u\rightarrow t}^2$ from $u$ to the destination node $t$, a partial path $P_{u\rightarrow t}$ is dominated by $P_{u\rightarrow t}^1$ and $P_{u\rightarrow t}^2$ if the following conditions hold:
\begin{enumerate}
    \item $d(P_{u\rightarrow t}^1)\leq d(P_{u\rightarrow t}) \leq d(P_{u\rightarrow t}^2)$;
    \item $d(P_{u\rightarrow t}^2) - d(P_{u\rightarrow t}^1)\leq U-L$;
    \item $c(P_{u\rightarrow t}^1)\leq c(P_{u\rightarrow t})$;
    \item $c(P_{u\rightarrow t}^2)\leq c(P_{u\rightarrow t})$.
\end{enumerate}
When $P_{u\rightarrow t}$ is dominated by $P_{u\rightarrow t}^1$ and $P_{u\rightarrow t}^2$, we can also say the delay-cost pair $(d(P_{u\rightarrow t}), c(P_{u\rightarrow t}))$ is dominated by $(d(P_{u\rightarrow t}^1),$ $c(P_{u\rightarrow t}^1))$ and $(d(P_{u\rightarrow t}^2),c(P_{u\rightarrow t}^2))$.
\end{definition}

Now we are ready to present the algorithm that computes the relaxed cost function. Starting from the destination node $t$, we perform the smallest-cost-first search using a min heap in the reverse direction. We represent each searching branch by a \emph{(node, delay, cost)} tuple, and this tuple means that there exist a path $P$ (which may contain cycles) from \emph{node} to the destination node $t$ such that $d(P)=\text{delay}$ and $c(P)=\text{cost}$. In lines 6-8 of Algorithm \ref{algorithm:relax_cost_function}, we perform the revised dominance check, and cut a branch if its delay-cost pair is dominated by those in previous branches. In lines 14-16 of Algorithm \ref{algorithm:relax_cost_function}, we perform the delay-based feasibility check, and cut a branch if it is not possible to obtain a path from the source node $s$ to the destination node $t$ that meets the delay upper bound. After the smallest-cost-first search, we obtain a list of delay-cost pairs for each node $u\in V$. Then, the relaxed cost function $f_u(l)$ can be calculated according to line 20 in Algorithm \ref{algorithm:relax_cost_function}. The correctness of Algorithm \ref{algorithm:relax_cost_function} is guaranteed by the following theorem.

\begin{algorithm}[t!]
\SetAlgoLined
\KwData{A network $G(V,E)$, a source node $s$, a destination node $t$, and a delay range $[L, U]$.}

\KwResult{The relax cost function $f_u$ for every $u\in V$.}

%\tcp{Basic definitions.}
Define a $Z=(\text{node, delay, cost})$ tuple. Given $Z_1$ and $Z_2$, define $Z_1 < Z_2$ if and only if $Z_1.\text{cost}<Z_2.\text{cost}$.

Define a min heap $H$ for the node-delay-cost tuple. Initialize $H=\{(t, 0, 0)\}$.

For every node $u\in V$, define a delay-cost pair set $\Pi_u$. Initialize $\Pi_u=\emptyset$.

\While{$H$ is not empty} {
    Let $(u, \text{delay\_to\_dst, cost\_to\_dst})=H.\text{pop()}$;
    
    \If{there exist two delay-cost pairs in $\Omega_u$ that dominate $(\text{delay\_to\_dst, cost\_to\_dst})$}{
        \textbf{continue};
    }

    $\Pi_u.\text{insert((delay\_to\_dst, cost\_to\_dst))}$;
    
    \For{every ingress link $e$ of the node $u$}{
        Let $v=\text{From}(e)$;
        
        Let $\text{new\_delay}=\text{delay\_to\_dst}+d(e)$;
        
        Let $\text{new\_cost}=\text{cost\_to\_dst}+c(e)$;
        
        \If{$\text{new\_delay}+d(P_{s\rightarrow v}^{\text{min\_delay}})\leq U$}{
            $H.\text{push}((v, \text{new\_delay}, \text{new\_cost}))$;
        }
    }
}

\For{each node $u$ and each delay value $l$}{
    Compute $f_u(l)=\min\{c: \text{there exists } d\in [l, l+U-L] \text{ such that } (d,c)\in \Pi_u\}$;
}

\caption{Calculate $f_u$ According to (\ref{eqn:relaxed_cost_function})}
\label{algorithm:relax_cost_function}
\end{algorithm}

\begin{theorem}\label{thm:relax_cost_function}
For every node $u$ and every delay value $l\leq L-d(P_{s\rightarrow u}^{\text{min\_delay}})$, the $f_u(l)$ computed by Algorithm \ref{algorithm:relax_cost_function} is equal to the relaxed cost function defined by (\ref{eqn:relaxed_cost_function}).
\end{theorem}

% \todo{我在想是不是可以把剪枝条件提到前面的位置，就是说，在介绍完cut node之后，从两个角度分析为什么会被cut掉，第一个角度是按照feasibility check， 第二个角度是dominance check}

\begin{table*}[t]
\centering
\caption{Evaluating joint delay \& cost pruning strategy for Pulse$+$.}
\label{tab:separate_vs_joint}
\begin{tabular}{|c|c|c|c|c|}
\hline
\multirow{2}{*}{Test Cases} & Pulse$+$ w/o Joint Pruning & \multicolumn{3}{c|}{Pulse$+$ w/ Joint Pruning } \\
                  & Ave. Run Time   & Ave. Run Time & Ave. Init Time & Ave. Total Time \\
\hline
DRCR\_1         & 12.0159 $\mu s$  & 10.5622 $\mu s$  & 2439.19 $\mu s$  & 2449.75 $\mu s$  \\
\hline
DRCR\_2         & 10886.7 $\mu s$   & 7270.08 $\mu s$  & 21464.18 $\mu s$  & 28734.26 $\mu s$  \\
\hline
\end{tabular}
\end{table*}

\begin{proof}
When $l< d(P_{u\rightarrow t}^{\text{min\_delay}})-U+L$, there exists no path from the node $u$ to the destination node $t$. In this case, the values of $f_u(l)$ computed by Algorithm \ref{algorithm:relax_cost_function} and Equation (\ref{eqn:relaxed_cost_function}) are both $+\infty$.

When $d(P_{u\rightarrow t}^{\text{min\_delay}})-U+L\leq l\leq L-d(P_{s\rightarrow u}^{\text{min\_delay}})$, let $\mathcal{P}_{u \rightarrow t}$ be the set of paths that attain the smallest end-to-end cost among all paths whose end-to-end delays are within $[l, l+U-L]$. We only need to prove that there exist a path $P_{u\rightarrow t}\in \mathcal{P}_{u\rightarrow t}$ such that $(d(P_{u\rightarrow t}), c(P_{u\rightarrow t}))\in\Pi_u$.

We prove by contradiction. Assume that there exists no path $P_{u\rightarrow t}\in \mathcal{P}_{u\rightarrow t}$ such that $(d(P_{u\rightarrow t})$, $c(P_{u\rightarrow t}))\in\Pi_u$. For every path $P_{u\rightarrow t}\in \mathcal{P}_{u\rightarrow t}$, let $u_1=u, u_2, u_3,..., u_K=t$ be the sequence of nodes visited by the path $P_{u\rightarrow t}$, and let $P_{u_i\rightarrow u_j}^{\text{sub}}$ be the sub-path of $P_{u\rightarrow t}$ from $u_i$ to $u_j$. Since $(d(P_{u\rightarrow t}), c(P_{u\rightarrow t}))\notin\Pi_u$, there must exist a node $u_k$ such that the branch $P_{u_k\rightarrow t}^{\text{sub}}$ is cut by Algorithm \ref{algorithm:relax_cost_function}. We call the node $u_k$ as the \textbf{cut node} of the path $P_{u\rightarrow t}$. Among all the paths in $\mathcal{P}_{u\rightarrow t}$, we consider the path $P_{u\rightarrow t}^*$ whose \textbf{cut node} is closest to the node $u$ in terms of the hop count along the same path. We will derive contradictions based on $P_{u\rightarrow t}^*$.

\noindent\textbf{Step 1:} We first check whether the branch $P_{u_k^*\rightarrow t}^{\text{sub}}$($u_k^*$ is the \textbf{cut node} of the path $P_{u\rightarrow t}^*$) is cut by the feasibility check in lines 14-16 of Algorithm \ref{algorithm:relax_cost_function}. Since
% \begin{eqnarray}
% &&d(P_{s\rightarrow u_k}^{\text{min\_delay}})+d(P_{u_k^*\rightarrow t}^{\text{sub}})\leq d(P_{s\rightarrow u}^{\text{min\_delay}})+d(P_{u\rightarrow t}^*)\nonumber\\
% &\leq& d(P_{s\rightarrow u}^{\text{min\_delay}})+l+U-L\leq U,\nonumber
% \end{eqnarray}
$$\begin{aligned}
&d(P_{s\rightarrow u_k}^{\text{min\_delay}})+d(P_{u_k^*\rightarrow t}^{\text{sub}})
\leq d(P_{s\rightarrow u}^{\text{min\_delay}})+d(P_{u\rightarrow t}^*)\\
\leq & d(P_{s\rightarrow u}^{\text{min\_delay}})+l+U-L\leq U,\end{aligned}$$
it doesn't meet the requirement of the feasibility check. Hence, the branch $P_{u_k^*\rightarrow t}^{\text{sub}}$ cannot be cut by the feasibility check. 

\noindent\textbf{Step 2:} We then check the possibility of this branch being cut by the dominance check in lines 6-8 of Algorithm \ref{algorithm:relax_cost_function}. Consider the delay interval $I=[d(P_{u_k^*\rightarrow t}^{\text{sub}})-d(P_{u\rightarrow t}^*)+l, d(P_{u_k^*\rightarrow t}^{\text{sub}})-d(P_{u\rightarrow t}^*)+l+U-L]$. Since $d(P_{u\rightarrow t}^*)\in [l, l+U-L]$, it is easy to verify that $d(P_{u_k^*\rightarrow t}^{\text{sub}})\in I$. Since the branch $P_{u_k^*\rightarrow t}^{\text{sub}}$ is cut by the dominance check, there must exist another path $P_{u_k^*\rightarrow t}^'$ such that $d(P_{u_k^*\rightarrow t}^{'})\in I$, $c(P_{u_k^*\rightarrow t}^{'})\leq c(P_{u_k^*\rightarrow t}^{\text{sub}})$ and $P_{u_k^*\rightarrow t}^'$ is not cut at the node $u_k^*$. Since $d(P_{u_k^*\rightarrow t}^{'})\in I$, if we concatenate the sub-path $P_{u\rightarrow u_k^*}^{\text{sub}}$ with $P_{u_k^*\rightarrow t}^{'}$ and denote this path as $P_{u\rightarrow t}^{'}$, then
$$d(P_{u\rightarrow t}^{'})=d(P_{u_k^*\rightarrow t}^{'}) + d(P_{u\rightarrow t}^*)-d(P_{u_k^*\rightarrow t}^{\text{sub}})\in [l,l+U-L].$$
We derive contradictions in two cases. 
\begin{description}
\item[Case 1:]$c(P_{u_k^*\rightarrow t}^{'})<c(P_{u_k^*\rightarrow t}^{\text{sub}})$. Since
% \begin{eqnarray}
% c(P_{u\rightarrow t}^{'})&=&c(P_{u_k^*\rightarrow t}^{'})+c(P_{u\rightarrow u_k^*}^{\text{sub}})\nonumber\\
% &<&c(P_{u_k^*\rightarrow t}^{\text{sub}})+c(P_{u\rightarrow u_k^*}^{\text{sub}})=c(P_{u\rightarrow t}^*),\nonumber
% \end{eqnarray}
$$\begin{aligned}
& c(P_{u\rightarrow t}^{'})=c(P_{u_k^*\rightarrow t}^{'})+c(P_{u\rightarrow u_k^*}^{\text{sub}})\\
<&c(P_{u_k^*\rightarrow t}^{\text{sub}})+c(P_{u\rightarrow u_k^*}^{\text{sub}})=c(P_{u\rightarrow t}^*),\end{aligned}$$
we obtain a path $P_{u\rightarrow t}^{'}$ with lower cost than those in $\mathcal{P}_{u\rightarrow t}$, which contradicts to the definition of $\mathcal{P}_{u\rightarrow t}$.
\item[Case 2:]$c(P_{u_k^*\rightarrow t}^{'})=c(P_{u_k^*\rightarrow t}^{\text{sub}})$. In this case, $c(P_{u\rightarrow t}^{'})=c(P_{u\rightarrow t}^*),$ $d(P_{u\rightarrow t}^{'})\in [l,l+U-L]$. Thus, $P_{u\rightarrow t}^{'}\in \mathcal{P}_{u\rightarrow t}$. Now, consider the \textbf{cut node} of the path $P_{u\rightarrow t}^{'}$. Note that $P_{u\rightarrow t}^{'}$ is not cut at the node $u_k^*$, and $P_{u\rightarrow t}^{'},P_{u\rightarrow t}^{*}$ share the same sub-path from $u$ to $u_k^*$. The \textbf{cut node} of the path $P_{u\rightarrow t}^{'}$ must have a smaller hop count away from the node $u$ than the \textbf{cut node} $u_k^*$ of the path $P_{u\rightarrow t}^{*}$, which contradicts to the choice of the path $P_{u\rightarrow t}^{*}$.
\end{description}

We have proved that when $d(P_{u\rightarrow t}^{\text{min\_delay}})-U+L\leq l\leq L-d(P_{s\rightarrow u}^{\text{min\_delay}})$, there exists a path $P_{u\rightarrow t}\in \mathcal{P}_{u\rightarrow t}$ such that $(d(P_{u\rightarrow t}),$ $c(P_{u\rightarrow t}))\in\Pi_u$. Therefore, the $f_u(l)$ value calculated by Algorithm \ref{algorithm:relax_cost_function} is the same as that of Equation (\ref{eqn:relaxed_cost_function}).
\end{proof}

\subsection{Evaluating Joint Delay \& Cost Pruning Using the Relaxed Cost Function (\ref{eqn:relaxed_cost_function})}
We evaluate the effectiveness of the joint delay \& cost pruning strategy using the two synthetic problem sets DRCR\_1 and DRCR\_2. We compare the joint pruning strategy (\ref{eqn:joint_delay_cost_prune}) with the original pruning strategy (\ref{eqn:prune_strategy}) in Table \ref{tab:separate_vs_joint}. We can see that the joint pruning strategy reduces the average Pulse$+$ running time by about $12.5\%$ for DRCR\_1 and by about $33.2\%$ for DRCR\_2. However, preparing the relaxed cost function $f_u$ for joint pruning incurs significant overhead. Thus, whether to enable this optimization technique depends on the concrete use cases. If one just want to solve each DRCR problem instance once, we suggest using the original pruning strategy (\ref{eqn:prune_strategy}) in Pulse$+$. On the other hand, if one need to solve each DRCR problem multiple times, enabling joint delay \& cost pruning could be beneficial (see the CoSE-Pulse$+$ algorithm in Algorithm \ref{algorithm:cose_pulse}).

% \begin{figure}[!h]
%     \centering
%     \includegraphics[scale = 0.6]{images/sort_joint_table.pdf}
%     \caption{Evaluating joint delay \& cost pruning strategy for Pulse$+$.}
%     \label{fig:separate_vs_joint}
% \end{figure}
